# Supplementary material for: Geography-Aware Self-Supervised Learning
Source: arXiv:2011.09980 source file (2022-03-08)
Supplement: Supplementary file 1 [file appendix.tex]

%\newpage
\appendix
\section{Appendix}
% Please add the following required packages to your document preamble:
% \usepackage{booktabs}
\begin{table*}[!ht]
\resizebox{\textwidth}{!}{
\begin{tabular}{@{}|l|l|l|l|l|l|l|l|l|@{}}
\toprule
\textbf{Class Name}                      & \textbf{MoCo-v2 (Single)} & \textbf{MoCo-v2 (Temporal)} & \textbf{MoCo-v2 + Geo (Single)} & \textbf{MoCo-v2 + Geo (Temporal)} & \textbf{MoCo-v2 + TP (Single)} & \textbf{MoCo-v2 + TP (Temporal)} & \textbf{MoCo-v2 + Geo + TP (Single)} & \textbf{MoCo-v2+ Geo + TP (Temporal)} \\ \midrule
\textbf{airport}                         & 0.6858                    & 0.7                         & 0.7257                          & 0.7167                            & 0.8053                         & 0.7833                           & 0.6637                               & 0.7167                                \\ \midrule
\textbf{airport\_hangar}                 & 0.6159                    & 0.6816                      & 0.441                           & 0.5475                            & 0.5861                         & 0.6927                           & 0.5747                               & 0.6536                                \\ \midrule
\textbf{airport\_terminal}               & 0.4791                    & 0.4756                      & 0.4975                          & 0.5366                            & 0.6147                         & 0.6585                           & 0.5678                               & 0.622                                 \\ \midrule
\textbf{amusement\_park}                 & 0.6832                    & 0.7411                      & 0.7195                          & 0.7614                            & 0.7666                         & 0.8376                           & 0.7013                               & 0.7665                                \\ \midrule
\textbf{aquaculture}                     & 0.7737                    & 0.8243                      & 0.8848                          & 0.8784                            & 0.8148                         & 0.8378                           & 0.7819                               & 0.8378                                \\ \midrule
\textbf{archaeological\_site}            & 0.2608                    & 0.2869                      & 0.4113                          & 0.4918                            & 0.4032                         & 0.459                            & 0.4328                               & 0.5                                   \\ \midrule
\textbf{barn}                            & 0.4333                    & 0.52                        & 0.6131                          & 0.7                               & 0.5821                         & 0.66                             & 0.5762                               & 0.6743                                \\ \midrule
\textbf{border\_checkpoint}              & 0.1093                    & 0.0943                      & 0.2429                          & 0.2264                            & 0.3077                         & 0.3396                           & 0.2429                               & 0.2453                                \\ \midrule
\textbf{burial\_site}                    & 0.6032                    & 0.6724                      & 0.6128                          & 0.6782                            & 0.7408                         & 0.8161                           & 0.7008                               & 0.7989                                \\ \midrule
\textbf{car\_dealership}                 & 0.6364                    & 0.7554                      & 0.6453                          & 0.75                              & 0.6633                         & 0.7663                           & 0.6261                               & 0.6902                                \\ \midrule
\textbf{construction\_site}              & 0.1355                    & 0.15                        & 0.2191                          & 0.2875                            & 0.3147                         & 0.4375                           & 0.249                                & 0.3625                                \\ \midrule
\textbf{crop\_field}                     & 0.8971                    & 0.92                        & 0.9246                          & 0.9374                            & 0.9324                         & 0.9448                           & 0.9329                               & 0.9494                                \\ \midrule
\textbf{dam}                             & 0.7529                    & 0.8353                      & 0.743                           & 0.8059                            & 0.8408                         & 0.8941                           & 0.7678                               & 0.8059                                \\ \midrule
\textbf{debris\_or\_rubble}              & 0.2                       & 0.3784                      & 0.2388                          & 0.5676                            & 0.2597                         & 0.5135                           & 0.2687                               & 0.5946                                \\ \midrule
\textbf{educational\_institution}        & 0.5803                    & 0.6208                      & 0.5                             & 0.5874                            & 0.497                          & 0.5613                           & 0.4898                               & 0.5613                                \\ \midrule
\textbf{electric\_substation}            & 0.7209                    & 0.7933                      & 0.6349                          & 0.7308                            & 0.8023                         & 0.875                            & 0.7535                               & 0.8558                                \\ \midrule
\textbf{factory\_or\_powerplant}         & 0.2943                    & 0.4103                      & 0.3528                          & 0.4274                            & 0.3748                         & 0.453                            & 0.4333                               & 0.5214                                \\ \midrule
\textbf{fire\_station}                   & 0.1644                    & 0.164                       & 0.3043                          & 0.3545                            & 0.3668                         & 0.3862                           & 0.25                                 & 0.2804                                \\ \midrule
\textbf{flooded\_road}                   & 0.408                     & 0.425                       & 0.4417                          & 0.5625                            & 0.5429                         & 0.5375                           & 0.5706                               & 0.6875                                \\ \midrule
\textbf{fountain}                        & 0.6972                    & 0.7468                      & 0.7758                          & 0.8038                            & 0.804                          & 0.8608                           & 0.7746                               & 0.8608                                \\ \midrule
\textbf{gas\_station}                    & 0.4956                    & 0.5732                      & 0.5057                          & 0.5427                            & 0.5997                         & 0.6768                           & 0.5769                               & 0.6646                                \\ \midrule
\textbf{golf\_course}                    & 0.8325                    & 0.9032                      & 0.8466                          & 0.914                             & 0.8995                         & 0.9462                           & 0.8642                               & 0.914                                 \\ \midrule
\textbf{ground\_transportation\_station} & 0.372                     & 0.4453                      & 0.5687                          & 0.6204                            & 0.643                          & 0.6788                           & 0.5961                               & 0.6715                                \\ \midrule
\textbf{helipad}                         & 0.4653                    & 0.5357                      & 0.6319                          & 0.7143                            & 0.65                           & 0.7214                           & 0.6028                               & 0.7                                   \\ \midrule
\textbf{hospital}                        & 0.1195                    & 0.102                       & 0.153                           & 0.1497                            & 0.2378                         & 0.2517                           & 0.1427                               & 0.1429                                \\ \midrule
\textbf{impoverished\_settlement}        & 0.6166                    & 0.6667                      & 0.6995                          & 0.7273                            & 0.772                          & 0.8182                           & 0.6736                               & 0.7879                                \\ \midrule
\textbf{interchange}                     & 0.8035                    & 0.878                       & 0.8579                          & 0.9024                            & 0.8825                         & 0.939                            & 0.8175                               & 0.9268                                \\ \midrule
\textbf{lake\_or\_pond}                  & 0.3619                    & 0.4545                      & 0.5619                          & 0.6364                            & 0.4857                         & 0.5682                           & 0.4381                               & 0.5227                                \\ \midrule
\textbf{lighthouse}                      & 0.6032                    & 0.7219                      & 0.7275                          & 0.7815                            & 0.7495                         & 0.7947                           & 0.6934                               & 0.7682                                \\ \midrule
\textbf{military\_facility}              & 0.5258                    & 0.5742                      & 0.5365                          & 0.5871                            & 0.5737                         & 0.6032                           & 0.5752                               & 0.6387                                \\ \midrule
\textbf{multi-unit\_residential}         & 0.2538                    & 0.2211                      & 0.335                           & 0.3317                            & 0.4501                         & 0.397                            & 0.4171                               & 0.402                                 \\ \midrule
\textbf{nuclear\_powerplant}             & 0.5312                    & 0.7                         & 0.2812                          & 0.4                               & 0.5938                         & 0.8                              & 0.5938                               & 0.8                                   \\ \midrule
\textbf{office\_building}                & 0.2515                    & 0.2781                      & 0.072                           & 0.0651                            & 0.1685                         & 0.1716                           & 0.149                                & 0.1361                                \\ \midrule
\textbf{oil\_or\_gas\_facility}          & 0.5                       & 0.5911                      & 0.6807                          & 0.749                             & 0.69                           & 0.7328                           & 0.676                                & 0.7328                                \\ \midrule
\textbf{park}                            & 0.4758                    & 0.5536                      & 0.5311                          & 0.5804                            & 0.6321                         & 0.6696                           & 0.538                                & 0.5804                                \\ \midrule
\textbf{parking\_lot\_or\_garage}        & 0.4728                    & 0.5263                      & 0.4636                          & 0.5239                            & 0.5995                         & 0.6316                           & 0.4923                               & 0.5335                                \\ \midrule
\textbf{place\_of\_worship}              & 0.4624                    & 0.5543                      & 0.7154                          & 0.7888                            & 0.6327                         & 0.7112                           & 0.6674                               & 0.7236                                \\ \midrule
\textbf{police\_station}                 & 0.1494                    & 0.1768                      & 0.1195                          & 0.1463                            & 0.1896                         & 0.2256                           & 0.1883                               & 0.2195                                \\ \midrule
\textbf{port}                            & 0.8872                    & 0.913                       & 0.8083                          & 0.8116                            & 0.797                          & 0.8696                           & 0.8195                               & 0.7971                                \\ \midrule
\textbf{prison}                          & 0.5196                    & 0.6224                      & 0.5024                          & 0.5714                            & 0.6421                         & 0.6633                           & 0.6028                               & 0.6531                                \\ \midrule
\textbf{race\_track}                     & 0.7065                    & 0.7697                      & 0.671                           & 0.7135                            & 0.7598                         & 0.7865                           & 0.7811                               & 0.8202                                \\ \midrule
\textbf{railway\_bridge}                 & 0.5926                    & 0.6783                      & 0.7151                          & 0.7913                            & 0.7422                         & 0.8174                           & 0.7479                               & 0.8435                                \\ \midrule
\textbf{recreational\_facility}          & 0.8634                    & 0.9181                      & 0.8627                          & 0.9181                            & 0.8965                         & 0.9356                           & 0.8717                               & 0.9208                                \\ \midrule
\textbf{road\_bridge}                    & 0.6592                    & 0.7654                      & 0.7276                          & 0.8395                            & 0.806                          & 0.8951                           & 0.7251                               & 0.8457                                \\ \midrule
\textbf{runway}                          & 0.6791                    & 0.7156                      & 0.7059                          & 0.7706                            & 0.746                          & 0.7523                           & 0.7433                               & 0.7431                                \\ \midrule
\textbf{shipyard}                        & 0.1053                    & 0.0556                      & 0.3158                          & 0.4444                            & 0.1579                         & 0.1667                           & 0.2368                               & 0.2778                                \\ \midrule
\textbf{shopping\_mall}                  & 0.4584                    & 0.4895                      & 0.5194                          & 0.5804                            & 0.5461                         & 0.6154                           & 0.5216                               & 0.6014                                \\ \midrule
\textbf{single-unit\_residential}        & 0.743                     & 0.7683                      & 0.4985                          & 0.5317                            & 0.6406                         & 0.661                            & 0.6015                               & 0.6317                                \\ \midrule
\textbf{smokestack}                      & 0.4781                    & 0.5818                      & 0.534                           & 0.6364                            & 0.6929                         & 0.7818                           & 0.5946                               & 0.6636                                \\ \midrule
\textbf{solar\_farm}                     & 0.7658                    & 0.8717                      & 0.8291                          & 0.9211                            & 0.8434                         & 0.9408                           & 0.856                                & 0.9441                                \\ \midrule
\textbf{space\_facility}                 & 0.3636                    & 0.5                         & 0.3864                          & 0.5                               & 0.4318                         & 0.5                              & 0.4091                               & 0.25                                  \\ \midrule
\textbf{stadium}                         & 0.7376                    & 0.7526                      & 0.6983                          & 0.7216                            & 0.8185                         & 0.8351                           & 0.7561                               & 0.7629                                \\ \midrule
\textbf{storage\_tank}                   & 0.8164                    & 0.8324                      & 0.8474                          & 0.8844                            & 0.8963                         & 0.9191                           & 0.8617                               & 0.8786                                \\ \midrule
\textbf{surface\_mine}                   & 0.6863                    & 0.7722                      & 0.6582                          & 0.7606                            & 0.7694                         & 0.8417                           & 0.7265                               & 0.8031                                \\ \midrule
\textbf{swimming\_pool}                  & 0.6402                    & 0.7368                      & 0.7273                          & 0.8618                            & 0.7964                         & 0.8816                           & 0.7747                               & 0.8684                                \\ \midrule
\textbf{toll\_booth}                     & 0.7906                    & 0.8901                      & 0.8412                          & 0.8956                            & 0.8797                         & 0.9341                           & 0.8773                               & 0.9341                                \\ \midrule
\textbf{tower}                           & 0.4867                    & 0.5993                      & 0.4384                          & 0.5699                            & 0.6269                         & 0.6949                           & 0.5852                               & 0.7022                                \\ \midrule
\textbf{tunnel\_opening}                 & 0.8702                    & 0.9531                      & 0.8851                          & 0.9495                            & 0.9011                         & 0.9495                           & 0.8915                               & 0.9567                                \\ \midrule
\textbf{waste\_disposal}                 & 0.2695                    & 0.3643                      & 0.4253                          & 0.5039                            & 0.4692                         & 0.5504                           & 0.4172                               & 0.4961                                \\ \midrule
\textbf{water\_treatment\_facility}      & 0.685                     & 0.7866                      & 0.7735                          & 0.841                             & 0.7668                         & 0.8326                           & 0.7815                               & 0.8494                                \\ \midrule
\textbf{wind\_farm}                      & 0.8667                    & 0.927                       & 0.9373                          & 0.9831                            & 0.9307                         & 0.9747                           & 0.9438                               & 0.986                                 \\ \midrule
\textbf{zoo}                             & 0.3607                    & 0.4583                      & 0.459                           & 0.5625                            & 0.4877                         & 0.5833                           & 0.4672                               & 0.5208                                \\ \bottomrule
\end{tabular}}
\caption{Top 1 classification accuracies for different approaches on fMoW test set. We show the results on image classification and classification of images over time from an area. In the former case, we evaluate the models w.r.t labels on images and in the latter case, we evaluate the models w.r.t labels on unique areas.}
\label{tab:classwise}
\end{table*}
